# Supplementary material for: Flow-augmentation III: Complexity dichotomy for Boolean CSPs parameterized by the number of unsatisfied constraints
Source: arXiv:2207.07422 source file (2025-04-22)
Supplement: Supplementary file 1 [file appendix-algebra.tex]

\todo[inline]{MW: I worked out the following to scratch a personal
  itch. It's proof that there exists a type of algebraic condition
  which precisely characterizes the expressive power of proportional
  implementations. It follows that the FPT/W[1] tractability boundary
  can be described by these conditions (in particular, by a set of
  \emph{fractional polymorphisms with preconditions}). I do not yet
  have any useful concrete examples of such.}

\todo[inline]{
  A study of a \textsc{Boolean VCSP} dichotomy, for cost functions
  with non-negative (finite) integer costs, would probably benefit
  from being framed algebraically. The combinatorial mucking around
  with the graphs $G_R$ and $H_R$ can be expected to scale poorly
  to more complex settings.
}

\newcommand{\ar}{r}

Let $D$ be a finite domain and $\Gamma$ a finite-valued language over $D$.
For a function $f$ or relation $R$, let $\ar(f)$ respectively $\ar(R)$ denote the arity. 
Since our purpose is to analyze VCSP$(\Gamma)$ parameterized
by its natural parameter, we restrict our attention to cost functions
$f \colon D^{\ar(f)} \to \N$. A \emph{valued constraint} over $\Gamma$,
over a set of variables $V$, is an expression of the form $f(X)$
where $f \in \Gamma$ is the \emph{constraint function} and
$X \in V^{\ar(f)}$ is the \emph{scope} of the constraint.
Equivalently, if $X=(x_1,\ldots,x_{\ar(f)})$ we may write $f(X)=f(x_1,\ldots,x_{\ar(f)})$. 
We define a \emph{weighted formula} over $\Gamma$ with variable set $V=V(\cF)$
as an instance
\[
  \cF=\sum_{i=1}^m \beta_i f_i(X_i),
\]
where $f_i(X_i)$ is a valued constraint over $\Gamma$ and $V$
and $\beta_i \in \N$ is a weight.
The \emph{cost} in $\cF$ of an assignment $\alpha \colon V \to D$ is
\[
  f_{\cF}(\alpha) = \sum_{i=1}^m \beta_i f_i(\alpha(X_i)).
\]
The problem VCSP$(\Gamma)$ takes as input a weighted formula $\cF$ over
$\Gamma$ and an integer $k$, and asks whether there is an assignment
with cost at most $k$ in $\cF$. Note that in this setting, the weights $\beta_i$
are functionally equivalent to treating $\cF$ as a multiset of valued constraints.

The natural, 0/1-valued setting is when $\Gamma_0$ is a set of relations over $D$
(i.e., a non-valued constraint language), and we define a set $\Gamma$
of cost functions
\[
  f_R(x_1,\ldots,x_r) =
  \begin{cases}
    0 & (x_1,\ldots,x_r) \in R \\
    1 & \textrm{otherwise}.
  \end{cases}
\]
over relations $R \in \Gamma$, $r=\ar(R)$. Then \VCSP{\Gamma}
is equivalent to \MinCSP{\Gamma}. However, we consider
more general non-negative integer-valued cost functions
in order to allow for a more robust theory. 

We present two algebraic conditions. One, \emph{unbalanced fractional
  polymorphisms}, that corresponds directly to the expressive power
 of proportional implementations, and one, \emph{fractional
   polymorphisms with preconditions}, that is more specific to
 the needs of a parameterized complexity analysis.

\begin{definition} 
Let $f \colon D^r \to \mathbb{N}$ be a cost function and $\Gamma$ a constraint language.
A \emph{proportional implementation} of $f$ over $\Gamma$ 
is a formula $\cF$ over $\Gamma$, on a variable set $V(\cF)=X \cup Y$ where $|X|=r$,
such that
\[
c \cdot f(X) = \min_Y f_{\cF}(X,Y)
\]
holds for every $X \in D^r$, for some constant $c \in \mathbb{N}$, $c>0$. 
\end{definition}

\emph{Remark.} In terms of expressive power, there is no difference between
proportional implementations with positive integer costs and weights,
versus positive rational costs and weights. 
Instead of an integer coefficient $c$, 
we can consider any rational number $c=p/q$, $c>0$.
If $(p/q) \cdot f(X) = \min_Y f_{\cF}(X,Y)$
then $p \cdot f(X() = \min_Y f_{q \cdot \cF}(X,Y)$ where $q \cdot \cF$
represents taking $q$ disjoint copies of $\cF$. 
Similarly, if $\cF$ itself contains positive rational weights $\beta_i$,
then we can scale the entire implementation up by the least common multiple
of all denominators of the weights $\beta_i$, to get a weighted proportional
implementation using only integer weights and an integer scaling factor $c$. 
On the other hand, the requirement that all values are non-negative is essential.

\begin{definition}
  Let $\Psi^k$ for $k \geq 0$ be the set of all $k$-ary operations
  $p \colon D^k \to D$ over $D$, and let $\Psi=\bigcup_{k \geq 1} \Psi^k$. 
  A \emph{unbalanced fractional mapping} of arity $k$
  is a function $\omega \colon \Psi^k \to \Q_{\geq 0}$ such that
  $
    \sum_{p \in \Psi^k} \omega(p)\leq 1.
  $
  We say that $\omega$ is \emph{strictly unbalanced}
  if $\sum_{p \in \Psi^k} \omega(p) < 1$.
  Let $f \colon D^r \to \N$ be a cost function over $D$.
  An unbalanced fractional mapping $\omega$ of arity $k$
  is \emph{unbalanced fractional polymorphism} of $f$
  if, for every $\mathbf{x_1}, \ldots, \mathbf{x_k} \in D^r$, we have
  \[
    (1/k) \sum_{i=1}^k f(\mathbf{x_i}) \geq \sum_{p \in \Psi_k} \omega(p) f(p(\mathbf{x_1}, \ldots, \mathbf{x_k})).
  \]
  In this case, we say that $\omega$ \emph{improves} $f$. 
\end{definition}

\emph{Remark.} Let $f \colon D^r \to \N$ be a cost function.
If $\omega$ is an unbalanced fractional polymorphism
of $f$ and $\omega(p)>0$ then $p$ is a polymorphism of
the relation
$R_f=\{\mathbf{x} \in D^{\ar(f)} \mid f(\mathbf{x})=0\}$.
However, unlike the case of balanced fractional polymorphisms,
if $\min_{\mathbf{x}} f(\mathbf{x})=b>0$ then $p$
does not necessarily have to be a polymorphism of the set
of minimizing tuples $\{\mathbf{x} \in D^{\ar(f)} \mid f(\mathbf{x})=b\}$.
This is appropriate, since cost functions with only strictly positive
values are trivial to handle in an FPT algorithm for \VCSP{\Gamma}
by exhaustive branching. 

In the general-valued setting, where the range
of values is $\overline{\Q}=\Q \cup \{\infty\}$,
then $p$ also must be a polymorphism of the relation
defined by the set of finite-valued inputs of $f$.

\begin{lemma} \label{lemma:equals-unbalanced}
  Let $f$ be a finite-valued function and $\Gamma$ a finite,
  finite-valued language, over a finite domain $D$.  Then $f$ has a
  proportional implementation in $\Gamma$ if and only if every
  unbalanced fractional polymorphism of $\Gamma$ also improves $f$.
\end{lemma}
\begin{proof}
  In the one direction, it is easy to show that weighted sums and
  min-projections preserve unbalanced fractional polymorphisms.  We
  sketch the other direction. Let $n=\ar(f)$ and $k=|D|^n$. We claim
  that if there is a proportional implementation, then it suffices to
  use $|D|^k$ distinct variables. Indeed, let $\cF(X,Y)$ be a
  proportional implementation of $f(X)$. Then by definition
  $\cF(x,y) \geq f(x)$ for every assignment $(X,Y)=(x,y)$, and for
  every $x$ there exists a value $y_x$ such that $f(x)=\cF(x,y_x)$.
  Now, there are at most $|D|^k$ distinct columns $(y_x[i])_{x \in D^n}$,
  and if $y_x[i]=y_x[j]$ holds for $i \neq j$ for every $x$,
  then we can identify variables $i$ and $j$ and produce an
  implementation with fewer variables. Hence we can assume that there
  are st most $|D|^k$ variables in total.

  Now we have a finite number of possible constraints $f_i(Z)$ for
  valued functions $f_i \in \Gamma$ and variable tuples
  $Z \in (X \cup Y)^{\ar(f_i)}$, and each such constraint can be given
  a weight $\beta_{i,Z} \geq 0$. Hence we can set up an equation
  system with two conditions
  \[
    \sum_{i,Z} \beta_{i,Z} f_i(Z(x,y_x)) = f(x) \quad \forall x \in D^n
  \]
  and
  \[
    \sum_{i,Z} \beta_{i,Z} f_i(Z(x,y)) \geq f(x) \quad \forall (x,y) \in D^k.
  \]
  \todo{This is really just Farkas' lemma}
  Interpret this as a primal LP with optimization target $\min 0$
  (i.e., pure feasibility). The dual can be described as an LP over
  variables $p_x$ and $q_{x,y}$, with optimization target
  \[
    \max \sum_x p_x f_0(x) + \sum_{x,y} q_{x,y} f_0(x)
  \]
  given constraints
  \[
    \sum_x p_x f_i(Z(x,y_x)) + \sum_{x,y} q_{x,y} f_i(Z(x,y)) \leq 0
    \quad \forall (i,Z),
  \]
  where $p_x$ are free (potentially negative) variables and
  $q_{x,y} \geq 0$. If the primal is infeasible, then the dual is
  unbounded. In particular, there exists values for $p_x$ and
  $q_{x,y}$ satisfying the constraints with
  \[
    \sum_x p_x f_0(x) + \sum_{x,y} q_{x,y} f_0(x) > 0.
  \]
  Indeed, given such values we can scale $p_x$ and $q_{x,y}$ to
  increase the optimization value indefinitely.
  We claim that the values $p_x$ and $q_{x,y}$, correctly interpreted,
  defines an unbalanced fractional polymorphism that improves
  $\Gamma$ but not $f$. The arity of the fractional polymorphism is
  $k$, and each variable $q_{x,y}$ represents a function
  $g \colon D^k \to D$, by interpreting the indices $i \in [|D|^k]$
  of the vector $y$ as tabulating all tuples $t \in D^k$, and
  therefore $y$ tabulates an output $y[i]$ for every possible tuple 
  $t=(y_x[i])_{x \in D^n}$.

  Now, on the one hand select a function $f_i \in \Gamma$ of some
  arity $r$, and select an ``input'' consisting of rows (words)
  $w_1, \ldots, w_k \in D^r$. Write these as rows in a matrix. 
  Then there exist $r$ indices $j_1$, \ldots, $j_r$ such that
  for every $q \in [r]$, the tuple $(w_1[q],\ldots,w_k[q])$
  equals $(y_x[j_q])_{x \in D^n}$. Consider the pair $(i,Z)$
  where $Z=(j_1,\ldots,j_r)$. Then the values $p_x$ and $q_{x,y}$
  satisfy
  \[
    \sum_x p_x f_i(y_x[j_1], \ldots, y_x[j_r]) +
    \sum_{x,y} q_{x,y} f_i(y[j_1], \ldots, y[j_r]) \leq 0.
  \]
  Hence each $p_x$ gives a weight (potentially negative) 
  to a projection (i.e., corresponds to an evaluation of
  $f_i(w_j)$ for the index $j \in [k]$ corresponding to $x$);
  and every $q_{x,y}$ gives a non-negative weight to the function 
  tabulated by $y$. Hence $p_x$ and $q_{x,y}$ together define an
  unbalanced fractional polymorphism $\omega$ of $\Gamma$. In
  particular, if $\sum_x p_x + \sum_{x,y} q_{x,y}=0$ then we get a
  standard fractional polymorphism, but there is nothing in our
  equation system that guarantees this outcome. 

  On the other hand, the strictly positive goal function corresponds
  to the same calculation, for the function $f_0$ on the specific
  inputs $x_1, \ldots, x_k$ in the complete tabulation of $X$,
  showing that $f_0$ violates $\omega$.   
\end{proof}

However, there is a problem. Let an unbalanced fractional polymorphism
be \emph{trivial} if it improves every cost function, and \emph{strictly unbalanced}
if the weight on the two sides is different.

\begin{lemma}
  For every strictly unbalanced, non-trivial fractional polymorphisms $\omega$,
  there is a language $\Gamma$ that is not improved by $f$ but such that
  \MinCSP{\Gamma} is FPT.
\end{lemma}
\begin{proof}
  Let $D$ be the domain. Let $f \colon D^r \to \Q$ be a cost function
  not improved by $\omega$ (which exists by assumption). Then there is
  a constant $\varepsilon \geq 0$ such that $f'(x)=f(x)+\varepsilon$
  also violates $\omega$. Indeed, assume that $f$ violates $\omega$
  on some inputs $t_1, \ldots, t_n \in D^r$.
  Let $x=\sum_i (1/n)f(t_i)$ and $y=\sum_{p \in \omega} \omega(p) f(p(t_1,\ldots,t_n))$,
  hence $x < y$. Let $\xi = \sum_p \omega(p) < 1$ (since $\omega$ is strictly unbalanced).
  Let $x'$ and $y'$ be $x$ and $y$ evaluated on $f'$ instead of $f$.
  Then $x'=x+\varepsilon$ and $y'=y+\xi \varepsilon$.
  Hence $y'-x' = y-x-(1-\xi)\varepsilon$, and there exists some value
  $\varepsilon > 0$ such that the gap is still positive. 
  But now $f'$ is a cost function that never attains zero,
  and \VCSP{\Gamma} for such cost functions is trivially FPT. 
\end{proof}

\subsection{A stronger condition}

\begin{definition}
  Let $f \colon D^r \to \N$ be a cost function.
  A \emph{fractional mapping with $q$ preconditions}
  is an unbalanced fractional mapping $\omega$
  of some arity $k \geq q$ such that
  $\sum_p \omega(p) = 1-q/k$
  We say that $\omega$ is \emph{applicable} to
  a list of tuples $t_1, \ldots, t_k \in D^r$
  if $f(t_{k-q+1})=\ldots=f(t_k)=0$. 
  A \emph{fractional polymorphism with $q$ preconditions}
  is a fractional mapping $\omega$ with $q$ preconditions
  such that for every list of tuples
  $t_1, \ldots, t_k \in D^r$, if
  $\omega$ is applicable to the list
  then
  \[
    (1/k) \sum_{i=1}^{k} f(t_i) \geq \sum_p \omega(p) f(p(t_1,\ldots,t_k)).
  \]
\end{definition}

Note that the condition is effectively a balanced condition in cases where it is applicable. 
Indeed, if $\omega$ is applicable to $t_1, \ldots, t_k$ then
\[
  (1/k) \sum_{i=1}^k f(t_i) = (1-q/k) (1/(k-q)) \sum_{i=1}^{k-q} f(t_i)
  \geq \sum_p \omega(p) f(p(t_1,\ldots,t_k)),
\]
where $\sum_p \omega(p)=1-q/k$. Hence if we scale both sides by $(1-q/k)^{-1}$
we get the standard, balanced condition for a $(k-q)$-ary fractional polymorphism,
except that the right hand side may depend on $q$ further arguments as well.

We begin by noting that every unbalanced fractional polymorphism
implies a fractional polymorphism with precondition.

\begin{lemma} \label{lemma:turn-into-precond}
  Let $\omega$ be an unbalanced fractional polymorphism.  Then there
  is a fractional polymorphism $\omega'$ with $q$ preconditions (for any $q \geq 1$)
  such that for any cost function $f$, $\omega'$ improves $f$, for any cost function $f$, if and only if either
  $\omega$ improves $f$ or $\min_x f(x) > 0$. 
\end{lemma}
\begin{proof}
  Assume that $\omega$ is an operation of arity $k$, and let $\xi=\sum_p \omega(p)$
  be its weight. Create $\omega'$ by adding a single precondition $f(t_{k+1})$,
  letting $\omega'(e_{k+1})=(1-\xi)/(k+1)$ and $\omega'(p)=(k/(k+1))\omega(p)$
  for every other operation $p$.  Now $\omega'$ is a fractional polymorphism
  with 1 precondition. To reach $q$ preconditions, simply add $q-1$ further
  dummy arguments on the left-hand-sied and scale $\omega'$ accordingly.

  We show that $\omega'$ behaves as claimed. Assume that some cost function
  $f \colon D^r \to \N$ has a witness $t_1, \ldots, t_{k+1} \in D^r$ against
  $\omega'$. Then $f(t_{k+1})=0$, hence $\min_x f(x)=0$, and
  $t_1, \ldots, t_k$ is a witness against $\omega$.
 
  Conversely, let $t_1, \ldots, t_k \in D^r$ be a witness against $\omega$ for $f$
  and let $t_{k+1} \in D^r$ be such that $f(t_{k+1})=0$. Then $t_1, \ldots, t_{k+q}$
  forms a witness against $\omega'$. 
\end{proof} 

The converse is also true, for restricted types of unbalanced
fractional polymorphisms.

\begin{lemma} \label{lemma:equals-precondition}
  Let $\omega$ be a fractional mapping with $q$ preconditions and arity $k$.
  Let $e_i$ be the $i$:th $k$-ary projection. 
  For $\varepsilon > 0$, define $\omega_\varepsilon$ as the unbalanced fractional mapping where
  $\omega_\varepsilon(e_i)=(1-\varepsilon)/k+\varepsilon \omega(e_i)$ for every $1 \leq i \leq k-q$
  and $\omega_\varepsilon(p)=\varepsilon \omega(p)$ for every other operation $p$.
  Then $\omega$ is a fractional polymorphism of $f$ with $q$ preconditions
  if and only if there exists some $\varepsilon > 0$ such that $\omega_\varepsilon$
  is an unbalanced fractional polymorphism of $f$. 
\end{lemma}
\begin{proof}
  Consider the condition $\omega_\varepsilon$ for some $\varepsilon > 0$.
  We remark that the total weight of $\omega_\varepsilon$ is
  \[
    \sum_p \omega_\varepsilon(p) = ((k-q)/k)(1-\varepsilon) + \varepsilon \sum_p \omega(p),
  \]f
  i.e., an interpolation between the weight of $\omega(p)$ and the weight $1-q/k$. 
  Hence $\omega_\varepsilon$ is a valid unbalanced fractional mapping. 
  We have
  \[
    (1/k) \sum_{i=1}^k f(t_i) \geq (1-\varepsilon)/k \sum_{i=1}^{k-q} f(t_i) + \varepsilon \sum_p \omega(p) f(p(t_1,\ldots,t_k)),
  \]
  which, cancelling the common terms, becomes
  \[
    (1/k)(\sum_{i=1}^{k-q} \varepsilon f(t_i) + \sum_{i=k-q+1}^k f(t_i)) \geq \varepsilon \sum_p \omega(p) f(p(t_1,\ldots,t_k)).
  \]
  Scaling both sides by $N=1/\varepsilon$ for clarity we now get
  \[
    (1/k)\sum_{i=1}^k f(t_i) + \sum_{i=k-q+1}^k ((N-1)/k) f(t_i) \geq \sum_p \omega(p) f(p(t_1,\ldots,t_k)),
  \]
  i.e., the effect is precisely that of treating $\omega$ as a standard
  unbalanced fractional mapping, except that we also add
  $(N-1)/k \sum_{i=k-q+1}^k f(t_i)$ to the left-hand side of the condition.
  
  Let $f$ be an $r$-ary cost function over $D$, and 
  consider a list of tuples $t_1, \ldots, t_k  \in D^r$ that violates
  this condition of $\omega_\varepsilon$ for some $\varepsilon > 0$.
  There are two cases. If $f(t_i)>0$ for some $k-q+1 \leq i \leq k$,
  then clearly there is some $N>0$ such that adding $(N-1)f(t_i)$ to the
  left-hand side resolves the inequality. Hence there is a value $\varepsilon' > 0$
  for which all such violations are resolved. Then either
  there is a violation where $f(t_i)=0$ for every $k-q+1 \leq i \leq k$
  or not. If there is, then this list $t_1, \ldots, t_k$
  is a witness that $f$ violates $\omega$ with preconditions met,
  and the violation is unaffected by the value of $\varepsilon$
  (i.e., the same list violates $\omega_{\varepsilon'}$ for every $\varepsilon' > 0$).
  If there is no such witness, then by definition both $\omega_{\varepsilon'}$
  and $\omega$ improve $f$. 
\end{proof}

Note that every strictly positive cost function is improved by
every fractional mapping with $q$ preconditions as long as $q>0$. 
This has an implication for our notion of implementation. 

Let $\Gamma_+$ denote the set of all cost functions over $D$ which have
strictly positive costs.

\begin{lemma} \label{lemma:precond-is-preserved}
  Let $f$ be a cost function and $\Gamma$ a valued constraint language.
  Let $\omega$ be a fractional polymorphism of $\Gamma$ with $q>0$ preconditions.
  If $\Gamma \cup \Gamma_+$ has a proportional implementation of $f$,
  then $\omega$ improves $f$.
\end{lemma}
\begin{proof}
  Assume that $\Gamma \cup \Gamma_+$ has a proportional implementation
  of $f$. Let $\Gamma' \subset \Gamma \cup \Gamma_+$ be the cost
  functions actually used in the implementation; clearly $\Gamma'$ is
  finite. As noted, for every $f' \in \Gamma^+$, $\omega$ improves
  $f'$ vacuously. Hence $\omega$ is a fractional polymorphism
  of $\Gamma'$, and by Lemma~\ref{lemma:equals-precondition},
  for every $f' \in \Gamma'$ there is a value $\varepsilon > 0$
  such that $\omega_\varepsilon$ improves $f'$, and since $\Gamma'$
  is finite there is a value $\varepsilon > 0$ such that
  $\omega_{\varepsilon}$ is an unbalanced fractional polymorphism of
  $\Gamma'$. Since proportional implementations preserve unbalanced
  fractional polymorphisms, $\omega_\varepsilon$ also improves $f$.
  Now by Lemma~\ref{lemma:equals-precondition} $\omega$
  is a fractional polymorphism of $f$.
\end{proof}

We finally arrive at the following. 

\begin{lemma} \label{lemma:precond-condition}
  Let $\Gamma$ be a finite, finite-valued language over domain $D$
  and $f \colon D^r \to \N$. Then $f$ has a proportional
  implementation over $\Gamma \cup \Gamma_+$ if and only if
  there is no fractional polymorphism of $\Gamma$
  with $q \geq 1$ preconditions that is violated by $f$.
\end{lemma}
\begin{proof}
  If there is such a fractional polymorphism $\omega$, then by Lemma~\ref{lemma:precond-is-preserved}
  $f$ has no proportional implementation over $\Gamma \cup \Gamma_+$. 
  On other hand, assume that $f$ has no proportional implementation over $\Gamma \cup \Gamma_+$. 
  Then $\min_x f(x)=0$, as otherwise $f \in \Gamma_+$,
  and we note that cost functions $f' \in \Gamma_+$ are not useful for
  the implementation, as any implementation using $f'$ yields
  a cost function $f''$ with $\min_x f''(x)>0$. 
  By Lemma~\ref{lemma:equals-unbalanced} there is an unbalanced fractional
  polymorphism $\omega$ of $\Gamma$ that is violated by $f$.
  Since $\min_x f(X)=0$, by Lemma~\ref{lemma:turn-into-precond} there is a fractional polymorphism $\omega'$
  of $\Gamma$ with preconditions such that $f$ violates $\omega'$. 
\end{proof}
